# Supplementary material for: Overcoming Catastrophic Forgetting in Incremental Few-Shot Learning by Finding Flat Minima
Source: arXiv:2111.01549 source file (2021-11-04)
Supplement: Supplementary file 1 [file table_error.tex]

\begin{table*}[h]

\caption{The performance of F2M with 95\% confidence intervals.} 
\label{table:error}
\centering
\resizebox{\textwidth}{!}{
\begin{tabular}{lccccccccccc}
  \toprule
  \multirow[m]{2}{*}{\textbf{Dataset}} & \multicolumn{9}{c}{\textbf{sessions}}\\
  \cmidrule[0.05em]{2-12}
  & 1 & 2 & 3 & 4 & 5 & 6 & 7 & 8 & 9 & 10 & 11\\
  %%%%%%%%%%%%%%%%%%%%%%%%%%%%%%%%%%%%%%%%%%%%%%%%%%%%%%%%%%%%%%%%%%%%5
  \midrule
  \multirow{1}{*}[0.45em]{\textbf{CIFAR100}}                   & \multirow{1}{*}[0.5em]{64.71} & \shortstack[r]{62.05 \\ $\pm$ 0.19} & \shortstack[r]{59.01 \\ $\pm$ 0.22} & \shortstack[r]{55.58 \\ $\pm$ 0.21} & \shortstack[r]{52.55 \\ $\pm$ 0.25} & \shortstack[r]{49.96 \\ $\pm $ 0.30} & \shortstack[r]{48.08 \\ $\pm$ 0.24} & \shortstack[r]{46.28 \\ $\pm$ 0.24} & \shortstack[r]{44.67 \\ $\pm$ 0.23} & \multirow{1}{*}[0.5em]{-} & \multirow{1}{*}[0.35em]{-}\\
  \rule{0pt}{6ex}%
  \multirow{1}{*}[0.45em]{\textbf{miniImageNet}}               & \multirow{1}{*}[0.5em]{67.28} & \shortstack[r]{63.80 \\ $\pm$ 0.10} & \shortstack[r]{60.38 \\ $\pm$ 0.19} & \shortstack[r]{57.06 \\ $\pm$ 0.29} & \shortstack[r]{54.08 \\ $\pm$ 0.28} & \shortstack[r]{51.39 \\ $\pm$ 0.32} & \shortstack[r]{48.82\\ $\pm $ 0.32} & \shortstack[r]{46.58 \\ $\pm$ 0.33} & \shortstack[r]{44.65 \\ $\pm$ 0.29} & \multirow{1}{*}[0.5em]{-} & \multirow{1}{*}[0.35em]{-}\\
  \rule{0pt}{6ex}%
  \multirow{1}{*}[0.45em]{\textbf{CUB-200-2011}}               & \multirow{1}{*}[0.5em]{81.07} & \shortstack[r]{78.16 \\ $\pm$ 0.14} & \shortstack[r]{75.57 \\ $\pm$ 0.24} & \shortstack[r]{72.89 \\ $\pm$ 0.32} & \shortstack[r]{70.86 \\ $\pm$ 0.25} & \shortstack[r]{68.17 \\ $\pm $ 0.39} & \shortstack[r]{67.01 \\ $\pm$ 0.32} & \shortstack[r]{65.26 \\ $\pm$ 0.26} & \shortstack[r]{63.36 \\ $\pm$ 0.24} & \shortstack[r]{61.76\\ $\pm$ 0.27}   & \shortstack[r]{60.26 \\ $\pm$ 0.28} \\
  
  \bottomrule
\end{tabular}
}
\end{table*}

% %  & 67.28 & \textbf{63.80} & \textbf{60.38} & \textbf{57.06} & \textbf{54.08} & \textbf{51.39} & \textbf{48.82} & \textbf{46.58} & \textbf{44.65} & \textbf{-0.20}

%  \textbf{81.07} & \textbf{78.16} & \textbf{75.57} & \textbf{72.89} & \textbf{70.86} & \textbf{68.17} & \textbf{67.01} & \textbf{65.26} & \textbf{63.36} & \textbf{61.76} & \textbf{60.26} & \textbf{-0.82}\\
